# Supplementary material for: Trimming the Fat: Efficient Compression of 3D Gaussian Splats through Pruning
Source: arXiv:2406.18214 source file (2024-07-29)
Supplement: Supplementary file 1 [file supplementary.tex]

% \documentclass{bmvc2k}

% %% Enter your paper number here for the review copy
% \bmvcreviewcopy{358}

% \usepackage{graphicx}
% \usepackage{cleveref}
% \usepackage{multirow}
% \usepackage{algorithm}
% \usepackage{algpseudocode}
% \usepackage{booktabs}
% \usepackage{wrapfig}
% \usepackage{enumitem}
% \newcommand{\salman}[1]{\textcolor{blue}{#1}}
% \newcommand{\enzo}[1]{\textcolor{red}{#1}}




% \title{Supplementary Material for \\ Trimming the Fat: Efficient Compression of 3D Gaussian Splats through Pruning }

% % Enter the paper's authors in order
% % \addauthor{Name}{email/homepage}{INSTITUTION_CODE}
% \addauthor{Susan Student}{http://www.vision.inst.ac.uk/~ss}{1}
% \addauthor{Petra Prof}{http://www.vision.inst.ac.uk/~pp}{1}
% \addauthor{Colin Collaborator}{colin@collaborators.com}{2}

% % Enter the institutions
% % \addinstitution{Name\\Address}
% \addinstitution{
%  The Vision Institute\\
%  University of Borsetshire\\
%  Wimbleham, UK
% }
% \addinstitution{
%  Collaborators, Inc.\\
%  123 Park Avenue,\\
%  New York, USA
% }

% \runninghead{Student, Prof, Collaborator}{BMVC Author Guidelines}

% % Any macro definitions you would like to include
% % These are not defined in the style file, because they don't begin
% % with \bmva, so they might conflict with the user's own macros.
% % The \bmvaOneDot macro adds a full stop unless there is one in the
% % text already.
% \def\eg{\emph{e.g}\bmvaOneDot}
% \def\Eg{\emph{E.g}\bmvaOneDot}
% \def\etal{\emph{et al}\bmvaOneDot}

% %-------------------------------------------------------------------------
% % Document starts here
% \begin{document}

% \maketitle

% \begin{figure*}
% \includegraphics[width=\linewidth]{Figures/playroom_comparison.pdf}
%     \centering
%     \caption{Qualitative comparison of the playroom scene at various pruning levels, defined by $\gamma_{\text{iter}}$ using gradient-aware iterative pruning. Our proposed method demonstrates substantially higher compression rates compared to both baselines while maintaining similar visual quality.}
%     \label{fig: Pruning-Comparison-2}
%     %\vspace{-0.4cm}
% \end{figure*}


% \begin{figure*}
% \includegraphics[width=\linewidth]{Figures/train-pruning-comp.pdf}
%     \centering
%     \caption{Qualitative comparison of the \textit{train} scene at various pruning levels, defined by $\gamma_{\text{iter}}$ using gradient-aware iterative pruning. Our proposed method demonstrates substantially higher compression rates compared to both baselines while maintaining similar visual quality.}
%     \label{fig: Pruning-Comparison-3}
%     %\vspace{-0.4cm}
% \end{figure*}


% \begin{figure*}[t]
% \includegraphics[width=0.6\linewidth]{Figures/Tanks and Temple vs Compact3D.pdf}
%     \centering
%     \caption{The graph illustrates the performance-size trade-off achieved by our method compared to the pruning approach proposed in Compact 3D~\cite{lee2023compact} on the Tanks\&Temples dataset. }
%     \label{fig: ours vs compact}
%     %\vspace{-0.4cm}
% \end{figure*}


% \begin{table*}
    
%     \centering
%     \resizebox{\textwidth}{!}{
%     \begin{tabular}{l|c|cccc|cccc|cccc}
%     \toprule
%       &   & \multicolumn{4}{c}{Mip-NeRF360} & \multicolumn{4}{c}{Tanks\&Temples} & \multicolumn{4}{c}{Deep Blending} \\
%     \textbf{Model} & \textbf{$\gamma_{\text{iter}}$} & \textbf{SSIM$^\uparrow$} & \textbf{PSNR$^\uparrow$} & \textbf{LPIPS$^\downarrow$} & \textbf{Mem}$^\downarrow$ & \textbf{SSIM$^\uparrow$} & \textbf{PSNR$^\uparrow$} & \textbf{LPIPS$^\downarrow$} & \textbf{Mem}$^\downarrow$ & \textbf{SSIM$^\uparrow$} & \textbf{PSNR$^\uparrow$} & \textbf{LPIPS$^\downarrow$} & \textbf{Mem}$^\downarrow$ \\
%     \midrule
    
%    3DGS-7k$^\dag$& -   & 0.770 & 25.60 & 0.279 & 523.00 &0.767 & 21.20 & 0.280 & 270.00 & 0.875 & 27.78 & 0.317 & 386.00 \\
%     3DGS-30k$^\dag$& -     & 0.815 & 27.21 & 0.214 &    734.00   & 0.841 & 23.14 & 0.183 &  411.00  & 0.903 & 29.41 & 0.243 & 676.00 \\
%     3DGS-7k$^*$ & -    & 0.765 & 25.88 & 0.288 & 541.70  & 0.777 & 21.66 & 0.266 & 298.00 &  0.876 & 28.26 & 0.312 & 410.50  \\
%     3DGS-30k$^*$ & -     & 0.812 & 27.46 & 0.221 & 763.40  & 0.845 & 23.69 & 0.178 & 435.50 & 0.899 & 29.46 & 0.246 & 664.50 \\
% \midrule
%     \multirow{8}{*}{\begin{tabular}{@{}p{2cm}@{}}3DGS-Opacity Based\\Pruning\end{tabular}} & 0.025 & 0.813 & 27.58 & 0.217 & 592.22 & 0.849 & 23.98 & 0.169 & 338.50 & 0.894 & 29.27 & 0.248 & 516.00 \\
%     & 0.050 & 0.813 & 27.56 & 0.220 & 449.11 & 0.849 & 23.94 & 0.171 & 261.00 & 0.894 & 29.27 & 0.250 & 398.00 \\
%     & 0.075 & 0.809 & 27.47 & 0.231 & 344.00 & 0.846 & 23.96 & 0.178 & 200.00 & 0.895 & 29.27 & 0.252 & 305.00 \\
%     & 0.100 & 0.799 & 27.25 & 0.250 & 261.78 & 0.839 & 23.80 & 0.192 & 152.00 & 0.894 & 29.22 & 0.259 & 232.00 \\
%     & 0.150 & 0.762 & 26.46 & 0.304 & 148.00 & 0.818 & 23.40 & 0.232 & 86.00 & 0.888 & 28.96 & 0.279 & 131.00 \\
%     & 0.200 & 0.725 & 25.66 & 0.353 & 80.89 & 0.794 & 23.07 & 0.574 & 47.00 & 0.883 & 28.66 & 0.295 & 72.00 \\
%     & 0.250 & 0.692 & 24.98 & 0.394 & 42.78 & 0.767 & 22.66 & 0.310 & 25.00 & 0.877 & 28.20 & 0.310 & 38.00 \\
%     & 0.300 & 0.659 & 24.26 & 0.430 & 22.14 & 0.731 & 21.90 & 0.354 & 12.65 & 0.869 & 27.69 & 0.328 & 19.00 \\
% \midrule
%     \multirow{8}{*}{\begin{tabular}{@{}p{2cm}@{}}Trimming\\the Fat\end{tabular}} & 
%     0.225 & 0.813 & 27.60 & 0.217 & 543.44 & 0.849 & 23.96 & 0.170 & 335.50 & 0.898 & 29.50 & 0.247 & 534.00 \\
% & 0.275 & 0.814 & 27.60 & 0.219 & 464.33 & 0.849 & 23.97 & 0.171 & 280.75 & 0.898 & 29.48 & 0.247 & 481.50 \\
% & 0.325 & 0.813 & 27.60 & 0.223 & 386.11 & 0.848 & 23.97 & 0.175 & 219.25 & 0.899 & 29.51 & 0.248 & 416.00 \\
% & 0.375 & 0.810 & 27.57 & 0.231 & 311.78 & 0.844 & 23.94 & 0.187 & 153.00 & 0.899 & 29.53 & 0.250 & 339.00 \\
% & 0.450 & 0.797 & 27.35 & 0.256 & 194.22 & 0.829 & 23.85 & 0.220 & 76.75 & 0.899 & 29.55 & 0.253 & 205.50 \\
% & 0.500 & 0.776 & 26.93 & 0.288 & 119.44 & 0.810 & 23.56 & 0.251 & 45.25 & 0.899 & 29.52 & 0.258 & 116.00 \\
% & 0.550 & 0.740 & 26.21 & 0.336 & 63.56 & 0.780 & 22.92 & 0.294 & 23.38 & 0.897 & 29.25 & 0.269 & 59.00 \\
% & 0.600 & 0.690 & 25.03 & 0.394 & 29.22 & 0.761 & 22.51 & 0.319 & 14.75 & 0.887 & 28.66 & 0.293 & 25.50 \\
%     \bottomrule


    
%     \end{tabular}
%     }
%     \caption{Performance comparison using gradient-aware iterative pruning with different pruning levels defined by $\gamma$ against 3DGS-30k, 3DGS-7k baselines, and opacity-based iterative pruning. $^*$Reproduced using official code. $^\dag$ Reported from~\cite{kerbl20233d}. Memory size is in MBs.
%     %Comparison of performance using opacity-aware iterative pruning with different pruning levels defined by $\gamma$ against 3DGS-30k and 3DGS-7k baselines. $^*$Reproduced using official code. $^\dag$ Reported from \cite{kerbl20233d}. Memory size is in MBs.
%     %Comparison of performance using opacity-aware iterative pruning with different pruning levels defined by $\gamma$ against 3DGS-30k and 3DGS-7k baselines. $^*$Reproduced using official code. $^\dag$ Reported from \cite{kerbl20233d}. Memory size is in MBs
%     }
%     \label{tab:pruning_comp}
% \end{table*}


% %-------------------------------------------------------------------------
% \section{Additional Results}

% \subsection{Quantitative Comparison}
% Table~\ref{tab:pruning_comp} provides an extensive comparison between our proposed approach and the 3DGS-30k and 3DGS-7k baseline methods across various $\gamma_{\text{iter}}$ values. Across all datasets, our method demonstrates the potential to prune Gaussian splats up to 4$\times$ while achieving performance improvements or maintaining comparable levels to the baseline. Even at highly compressed rates ($\gamma_{\text{iter}}$ = 0.6), our approach delivers reasonable performance similar to that of 3DGS-7k, while achieving average compression ratios of approximately 24$\times$.



% \subsection{Qualitative Comparison}
% \label{sec:intro}
% We present visualizations of \textit{train} scene from the Tanks\&Temples dataset and \textit{playroom} scene from the Deep Blending dataset, all of which require substantial memory resources on average. In Fig~\ref{fig: Pruning-Comparison-2} and~\ref{fig: Pruning-Comparison-3}, we illustrate the visualizations of test set images at various pruning levels indicated by $\gamma_{\text{iter}}$. Our "trimming the fat" iterative pruning pipeline achieves noteworthy compression rates while maintaining comparable visual quality. Across all scenes depicted in the Fig.~\ref{fig: Pruning-Comparison-2} and~\ref{fig: Pruning-Comparison-3}, our method compresses the Gaussian splats by approximately $4\times$ with visual quality similar to 3DGS-30K. Furthermore, with $\gamma=0.60$, our method achieves an average compression ratio of approximately 12$\times$ while preserving visual quality comparable to 3DGS-7K.
%  \newpage
 
% \section{Additional Ablation Studies}

% \subsection{Lottery Ticket for the Gaussian Splats?}
%  We investigated the potential presence of a ``lottery ticket'' phenomenon~\cite{frankle2018lottery} for Gaussian splats. To test this hypothesis, we took an already pruned set of Gaussian splats from the Tanks\&Temples dataset and randomly reinitialized all learnable features, including spherical harmonics (SH) features, opacity, scale, and rotation. Subsequently, we attempted to train these Gaussian splats for 30,000 iterations, but they failed to converge. This experiment underscores the necessity of having a learned 3D prior to which redundant information can be pruned. It highlights the difficulty of training Gaussian splats with the minimum number of Gaussians without any prior information from the 3D scene.

% \subsection{Trimming the Fat vs Compact3D~\cite{lee2023compact}.} Fig.~\ref{fig: ours vs compact} depicts a comparison of PSNR and Gaussian counts between our proposed approach and Compact 3D using the Tanks\&Temples dataset. The results unequivocally highlight the superior performance of our method, demonstrating its capability to significantly reduce the number of Gaussians while maintaining baseline performance levels. These findings emphasize the effectiveness of our pruning technique and its potential to advance or replace existing compression methodologies for 3DGS.






% \bibliography{main}
% \end{document}
